# Supplementary material for: Extending and Evaluating and Novel Course Reform of introductory Mechanics
Source: arXiv:1112.5593 source file (2011-12-21)
Supplement: Supplementary file 1 [file app-cluster.tex]

\chapter{Cluster Analysis}\label{sec:clusteranalysis}

Cluster analysis aims to organize observations into subsets that are similar in some fashion. In our work, we are attempted to uncover subsets of students who made similar errors as measured through an empirically developed set of codes (Table \ref{tab:vpcodes}). By comparing the students' binary patterns we can determine on which groups of students have similar code patterns. Furthermore, we can evaluate if these subsets of students are characterized by some common underlying error or set of errors.

An $n \times m$ binary matrix $\mathbf{F}$ represents the affirmative nature of $m$ codes for $n$ students.

\begin{equation}
\mathbf{F} = \overbrace{\left.\begin{bmatrix} F_{11} & \cdots & F_{1j} & \cdots & F_{1m}  \\ \vdots & \ddots & \vdots &\ddots & \vdots \\ F_{i1} & \cdots & F_{ij} & \cdots & F_{im}  \\ \vdots & \ddots & \vdots &\ddots & \vdots \\ F_{n1} & \cdots & F_{nj} & \cdots & F_{nm} \end{bmatrix}\right\} \begin{rotate}{270}\text{Students}\end{rotate}}^\text{Codes}
\end{equation}

$F_{\cdot j}$ is the number of students who received an affirmative (1) to the $j^{th}$ code (out of $n$ students).

\begin{equation}
F_{\cdot j} = \sum_i^n F_{ij}
\end{equation}

 The $j^{th}$ column of $\mathbf{F}$ is a binary column vector; the elements of which represent whether or not a student received an affirmative mark (1) on the $j^{th}$ code.  The $i^{th}$ row of $\mathbf{F}$ is a binary row vector; the elements of which represent a code was marked as affirmative (1) for the $i^{th}$ student. We call this vector $\vec{S}_i$, the student vector. Each of the $n$ students has a corresponding $\vec{S}_i$.

\begin{equation}
\vec{S}_i = \begin{bmatrix} F_{i1} \hdots F_{ij} \hdots F_{nj} \end{bmatrix}
\end{equation}

The first step in our analysis is to determine which pairs of students have the most similar student vectors. Using some choice of metric, we compare the binary patterns between pairs of student vectors to identify which ones are most similar.

\section{Choosing  a Binary Distance Metric}\label{sec:bdm}

For cluster analyzing binary data, there are several metrics available. The literature recommends trying a few to ensure that the resulting clusters are either invariant to the metric chosen or easily interpretable \cite{clustereveritt}. 

The Hamming metric is the simplest choice for binary data. It defines the distance between student vectors $\vec{S}_{k}$ and $\vec{S}_{l}$ as the proportion of codes for which student $K$ and $L$ are inconsistent.

\begin{equation}\label{eqn:hamming}
D_{kl}^H = \frac{C_{kl}^{10} + C_{kl}^{01}}{C_{kl}^{11} + C_{kl}^{10} + C_{kl}^{01} + C_{kl}^{00}} = \frac{C_{kl}^{10} + C_{kl}^{01}}{n}
\end{equation}

Here $C_{kl}^{xy}$ represents the number of codes for which the $k^{th}$ and $l^{th}$ student received some mark $x$ and $y$ respectively. The superscripts ($xy$) indicate whether the code was marked affirmative (1) or negative(0). In the superscript, the first digit refers to  the $k^{th}$ student and the second digit refers to $l^{th}$ student. 

As an example, consider two student vectors $\vec{a} = [1 0 0 1 0 1]$ and $\vec{b} = [0 0 1 1 0 1]$. For these vectors, the inter-cluster distance is 1/3. Using Eq. \ref{eqn:hamming},

\begin{equation}\label{eqn:hammingex}
D_{ab}^H = \frac{C_{ab}^{10} + C_{ab}^{01}}{n} = \frac{1+1}{6} = \frac{1}{3}
\end{equation}

Computing this pairwise distance between all pairs of problems produces a $n \times n$ symmetric distance matrix, $\mathbf{D}^H$, with 0's along the diagonal. The elements of this matrix, $D^H_{kl}$, give the proportion of codes for which students $k$ and $l$ agree. The extrema of any one element are 0 (completely disagree) and 1 (completely agree).

The Jaccard metric is also a valid choice for binary data. It is somewhat similar to the Hamming metric expect that it neglects codes for which both students received negatives (0). The Jaccard metric defines the distance between student vectors $\vec{S}_{k}$ and $\vec{S}_{l}$ as the proportion of codes for which student $K$ and $L$ are disagree compared to the total number of codes minus those that are both negative.

\begin{equation}\label{eqn:jaccard}
D_{kl}^J = \frac{C_{kl}^{10} + C_{kl}^{01}}{C_{kl}^{11} + C_{kl}^{10} + C_{kl}^{01}} = \frac{C_{kl}^{10} + C_{kl}^{01}}{n- C_{kl}^{00}}
\end{equation}

Using the same example vectors, $\vec{a} = [1 0 0 1 0 1]$ and $\vec{b} = [0 0 1 1 0 1]$, we find the inter-cluster distance is 1/2. Generally speaking, inter-cluster distances are larger using the Jaccard metric. Using Eq. \ref{eqn:jaccard},

\begin{equation}\label{eqn:jaccardex}
D_{kl}^J = \frac{C_{kl}^{10} + C_{kl}^{01}}{n - C_{kl}^{00}} = \frac{1 + 1}{6 - 2} = \frac{1}{2}
\end{equation}

An $n \times n$ symmetric distance matrix with 0's along the diagonal, $\mathbf{D}^J$, is formed by computing this pairwise distance between all pairs of students. The elements of this matrix, $D^J_{kl}$, give Jaccard distance between $k^{th}$ and $l^{th}$ students The extrema of any one element are 0 (identical) and 1 (completely opposite).

\section{Forming Clusters}\label{sec:lf}
%
%\begin{figure}[ht]
%\centering
%\includegraphics[clip, trim = 8.7mm 7mm 7.3mm 7mm, width=0.75\columnwidth]{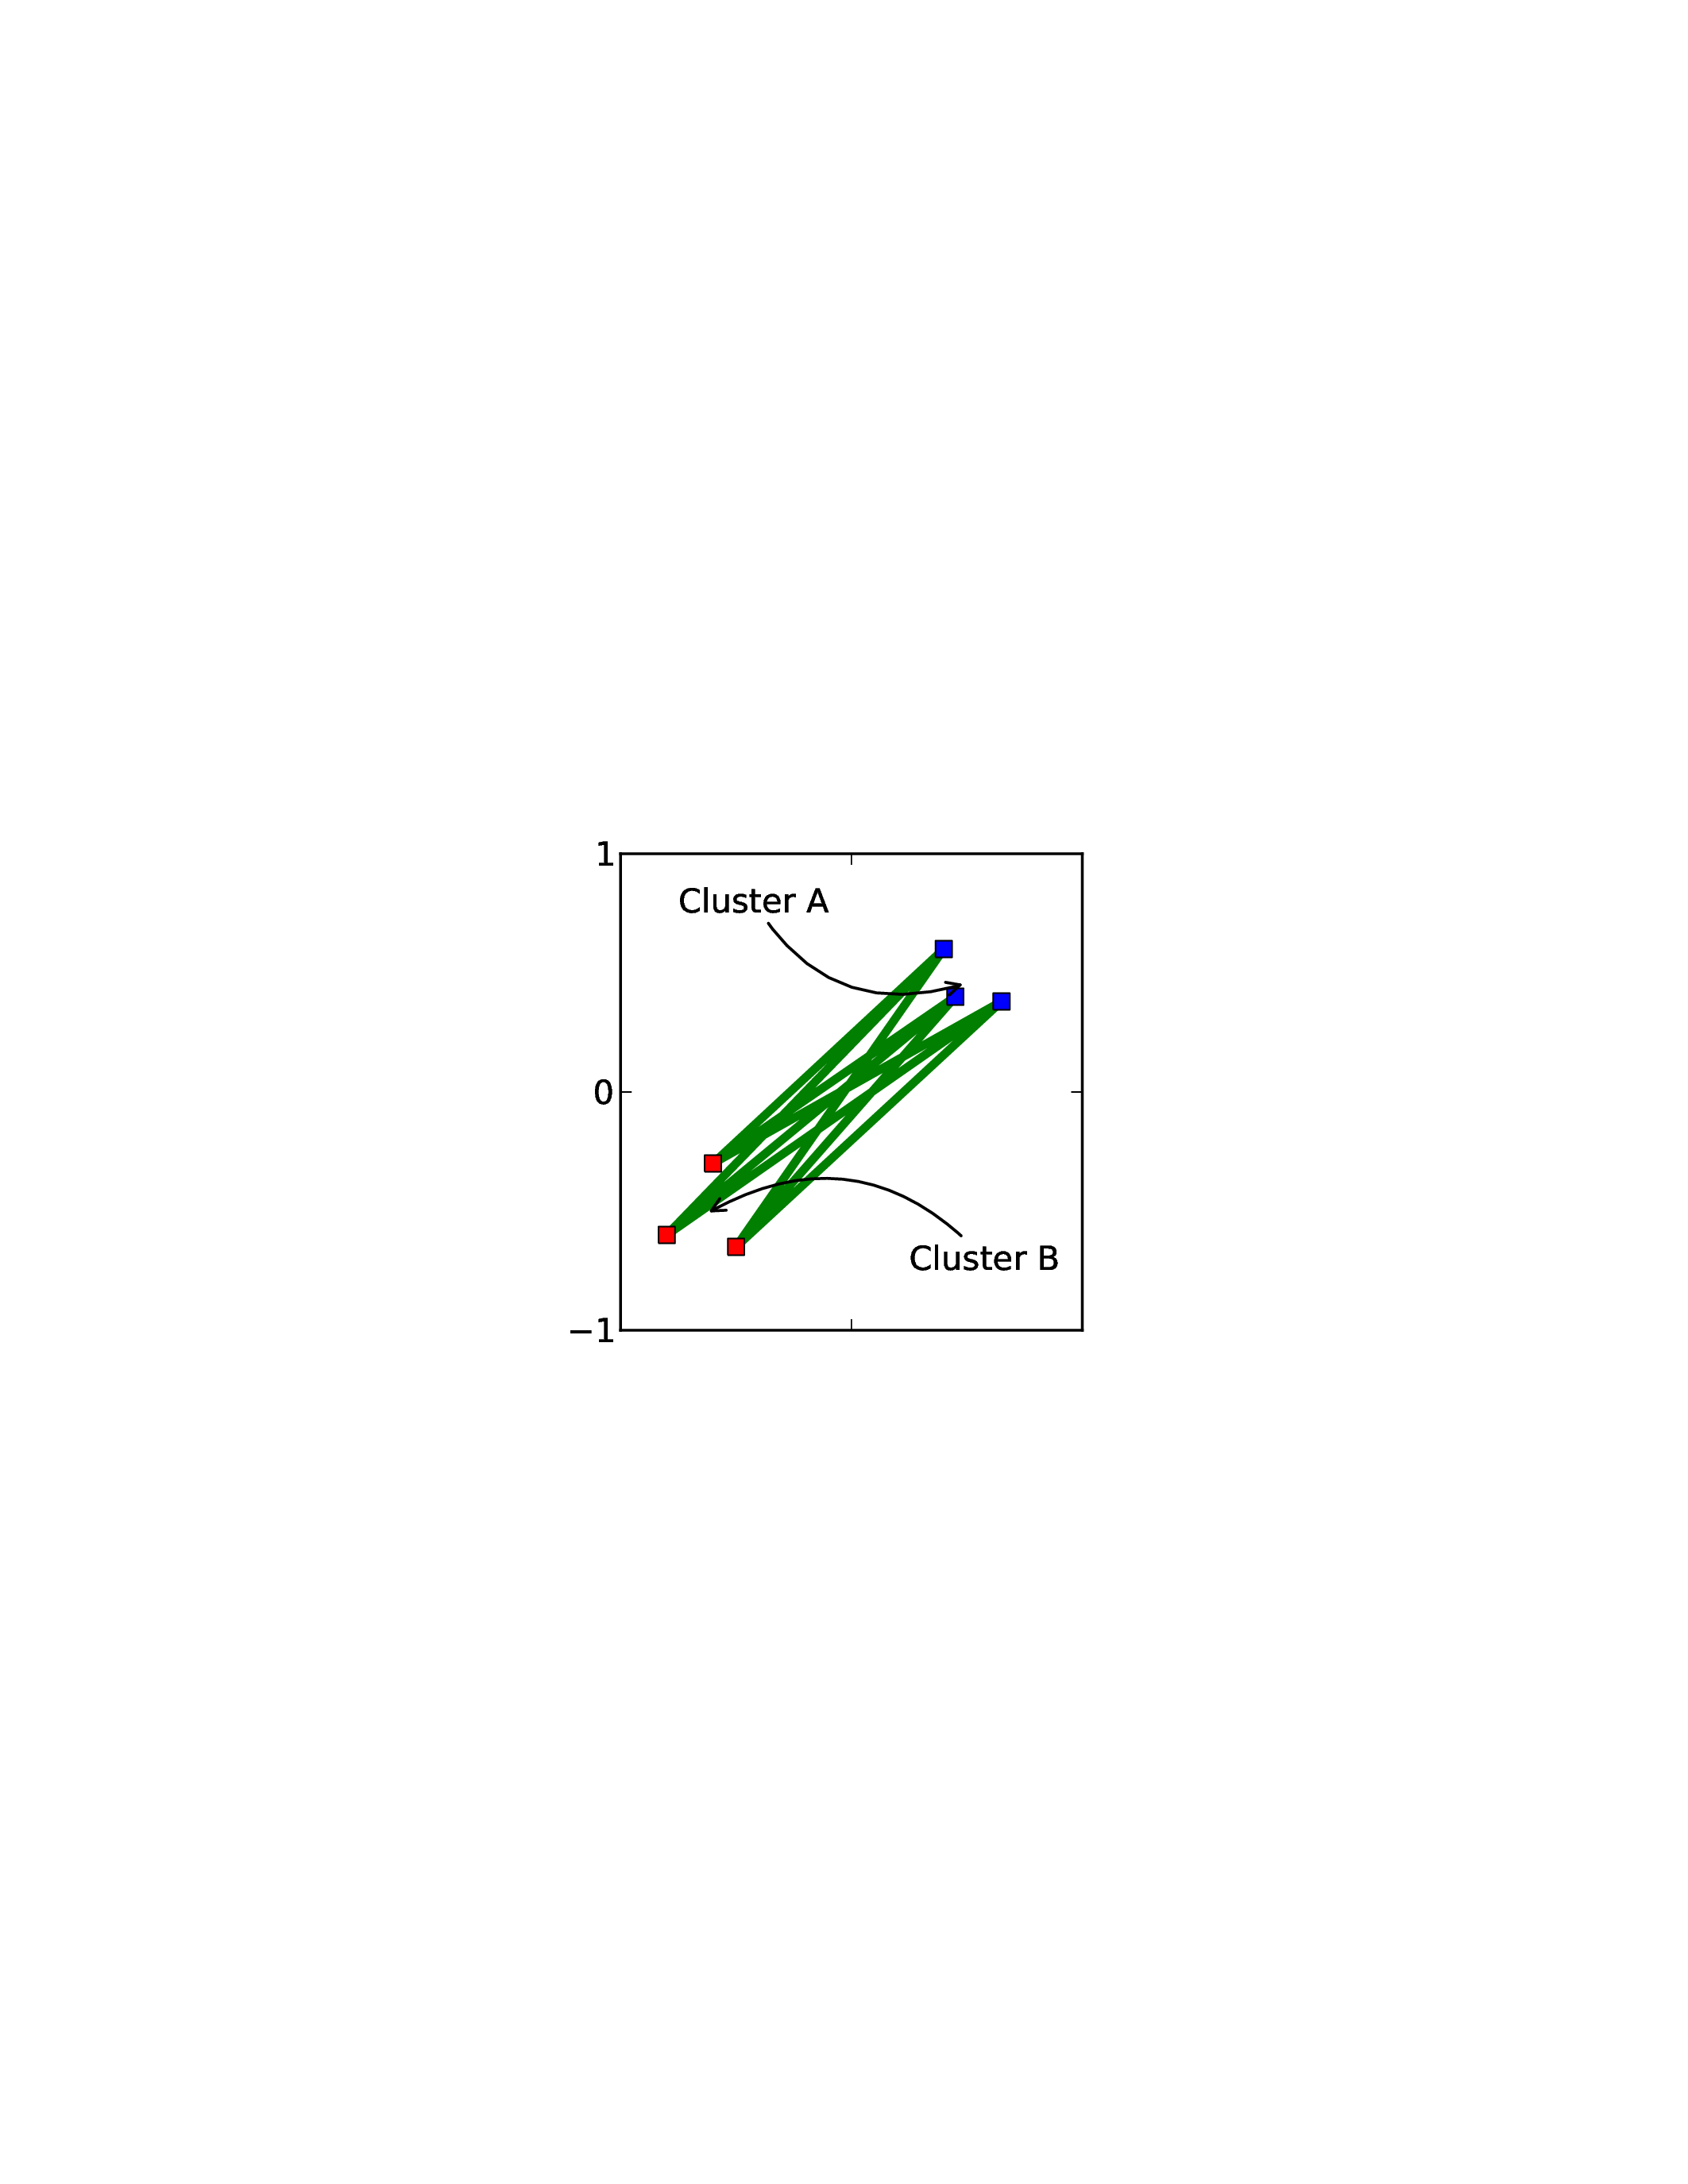}
%\caption{An illustration of using the average linkage function. The intercluster distance, $D(A,B)$, between two clusters is the mean distance between each element in a given cluster (Cluster A) and each element in another cluster (Cluster B). This linkage function takes into account the structure of the clusters.}\label{fig:clusterMeanLinkage}
%\end{figure}

After measuring the distance between problem vectors and constructing the distance matrix, we begin fusing problem vectors into clusters. Determining which problems (or clusters of problems) are fused is an iterative pair-wise process. First, the two problems with the smallest element in $\mathbf{D}^H$ are fused into a cluster. The cluster is treated as a single problem vector and distances from this cluster to all other problem vectors are remeasured. The new distances are computed using a linkage function.

Linkage functions determine how the new distances between clusters of problems, or intercluster distances, are computed. Several linkage functions exist: single linkage \cite{sneath1957application}, complete linkage \cite{sorenson1948method}, and average linkage \cite{sokal1975statistical}. We chose to use average linkage because it takes into account the structure of clusters and it is relatively robust \cite{clustereveritt}. The average linkage function computes the distance between clusters as the average distance between problems in the first cluster and problems in the second cluster. The intercluster distance between clusters $A$ and $B$ is given by,

\begin{equation}\label{eqn:avglink}
D(A,B) = \frac{1}{N_A N_B} \sum_{k \epsilon A} \sum_{l \epsilon B} D_{kl}^H
\end{equation}

where $N_A$ and $N_B$ are the number of problems in clusters $A$ and $B$ respectively. The intercluster distance defines the level at which clusters are fused and describes how ``close'' clusters are to each other. That is, it measures of the average proportion of students whose answers are inconsistent between problems in the cluster. For the present example, the intercluster distance, $D(A,B)$, is computed for each pair of clusters (or individual problem vectors) and those values form a new symmetric matrix, $\mathbf{D}^H_1$ which has been reduced to an $m-1 \times m-1$ matrix. The matrix is then searched again for the smallest element (corresponding to the closet pair of problem vectors or cluster and problem vector) and the resulting pair is forms the next cluster. The linkage function is used to compute the new intercluster distances between all pairs of clusters to form a reduced symmetrix matrix $\mathbf{D}^H_2$. The process repeats $m-1$ times until all problems are contained in single cluster. Throughout the procedure, we have kept track of which problems cluster at what intercluster distance.

Cluster analysis is a robust and diverse data classification technique. The above section was meant to give the reader a sense for how we used cluster analysis in our work; the interested reader is directed to the texts by Everitt \cite{clustereveritt}, Kaufmann \cite{clusterkaufman}, and Tan \cite{tan2006introduction}.

\section{Problem Clusters}\label{sec:questions}

Using the technique described in Sec. \ref{sec:clusteranalysis}, we analyzed both M\&I and traditional students' item scores on the FCI. The results are summarized by the dendrograms, Fig. \ref{fig:mi_cluster} and Fig. \ref{fig:trad_cluster}.

\subsection{Dendrograms}\label{sec:dendrograms}

Dendrograms are a visual representation of the cluster analysis procedure. Traditionally, the cluster variables (e.g., FCI problems) appear along the horizontal axis. The 30 vertical lines near the bottom of Figs. \ref{fig:mi_cluster} and \ref{fig:trad_cluster} represent each of the 30 problems on the FCI. In a typical dendrogram, horizontal lines appear that join vertical lines. These horizontal lines represent the fusion of cluster variables. These lines can join individual variables or clusters of variables. If two problems fuse to form a problem cluster, a single horizontal line connects the two vertical lines of those problems. The height of the horizontal line corresponds to the intercluster distance separating the two cluster variables. In our work, these horizontal lines represent the fraction of students whose responses are inconsistent between the pair of problems in the cluster. In Fig. \ref{fig:mi_cluster} there are 10 pairs of questions that cluster together in this fashion.

In addition to forming problem clusters from pairs of problems, it is possible that a single problem will cluster with an already formed cluster pair. In Fig. \ref{fig:mi_cluster}, we find this has happened with the clustered pair of problems 17 and 25 and the single problem 26. This clustering event occurs because the average distance from problem 26 to the cluster containing problems 17 and 25 is smaller than the distance between others pair of problems (e.g., problems 19 and 20). Horizontal lines represent the fusion of the clusters, but the height now measures the {\it average} fraction of students whose answers are inconsistent between all {\it pairs} of problems within the problem cluster.

Dendrograms provide an illustration of the iterative process of cluster analysis mentioned in Sec. \ref{sec:lf}. The reduction of the distance matrix is represented through the forming of links (horizontal lines) between problems (vertical lines) and problem clusters (vertical lines starting from a horizontal line). We can trace how problems fuse and which links are formed by starting from the bottom of the dendrogram and working upward.

\section{Comparing problem clusters}\label{sec:clustercompare}

Cluster sizes can range from one (i.e., all cluster variables in a single cluster) to the number of cluster variables in the analysis (i.e., each variable as its own cluster). The utility of cluster analysis is the organizing of items into some number of clusters which have meaning to the user (i.e., teacher or researcher). Because of the clustering algorithm, all items eventually form a single cluster. Selecting which clusters are ``real'' requires reviewing the variables in the formed clusters for common features. While this might appear subjective on the outset, the effect of ``chaining'' can be used to assist the user in his/her choice of clusters. There might be cluster variables that are far from most other variables that sequentially fuse to a particular cluster. On the average these problems are similar distances from that cluster, but not necessarily ``close''. That is, while the distances between the variables are mathematically similar, they might not have common features that are of interest to the user. 

In most cluster analyses, variables produce this chaining effect where individual cluster variables fuse one after another to a subset of variables. This effect is observed in Fig. \ref{fig:trad_cluster} where several problems (3,8,22,27) chain to a problem cluster near an intercluster distance of 0.3. Chaining occurs in all forms of cluster analysis but is most evident when intercluster distances become large. Chaining occurs more frequently when using the single linkage function \cite{clustereveritt}.
