# Supplementary material for: Extending and Evaluating and Novel Course Reform of introductory Mechanics
Source: arXiv:1112.5593 source file (2011-12-21)
Supplement: Supplementary file 2 [file app-comp-assessment.tex]

\chapter{Computational Modeling Assessment Tool}\label{app-comptool}
